# Supplementary material for: Multiple orbital contributions to molecular high-harmonic generation in an asymmetric top
Source: arXiv:1308.3733 source file (2013-08-16)
Supplement: Supplementary file 1 [file InversionSupp.pdf]

# Multiple orbital contributions to molecular high harmonic generation in an asymmetric top

*Supplementary Information*

LIMOR S. SPECTOR<sup>1,2\*</sup>, SHUNGO MIYABE<sup>2,3</sup>, ALVARO MAGANO<sup>4</sup>, SIMON PETRETTI<sup>4</sup>,  
PIERO DECLEVA<sup>5</sup>, TODD MARTINEZ<sup>2,3</sup>, ALEJANDRO SAENZ<sup>4</sup>  
MARKUS GUEHR,<sup>2</sup> AND PHILIP H. BUCKSBAUM<sup>1,2</sup>

<sup>1</sup> *Applied Physics Department, Stanford University, Stanford, CA 94305, USA*

<sup>2</sup> *Stanford PULSE Institute, SLAC National Accelerator Laboratory, Menlo Park, CA 94025, USA*

<sup>3</sup> *Chemistry Department, Stanford University, Stanford, CA 94305, USA*

<sup>4</sup> *Institut für Physik, Humboldt-Universität zu Berlin, Newtonstrasse 15, 12489 Berlin, Germany*

<sup>5</sup> *Dipartimento di Scienze Chimiche e Farmaceutiche and CNR-IOM Democritos and INSTM,*

*Università di Trieste, Via L. Giorgieri 1, I-34127 Trieste, Italy*

## I. ANALYSIS OF MULTIPLE ORBITALS

In the main text, we discuss the comparison of the theoretical and experimental contributions to high harmonic emission using a combination of the photoionization cross sections weighted by the field ionization calculations. However, in several prior papers [34,39-40], it was observed that the HHG cross spectrum was largely determined solely by the photoionization cross section, which models the recombination step of HHG. As a result, we examine here a comparison of the theoretical results of photoionization alone to a combination of photoionization and field ionization calculations.

Supplementary Fig. 1 is an expansion of Fig. 4 of the main text. As in Fig. 4, in Supplementary Fig. 1 we show the first few orbitals of SO<sub>2</sub> (HOMO through HOMO-5) with the orbital ordering obtained from Ref. 33. The rest of Supplementary Fig. 1 shows a comparison between harmonics 19 and 25, which are before and after the transition in the enhancement. The middle two columns display the relative contributions from each molecular axis in the experiment (top) and as calculated for photoionization only (bottom). Concentrating on the photoionization measurements for the moment, although the experiment shows the dominance of the b-axis (green) for the 19th harmonic, it shows a stronger contribution for the a-axis in the 25th harmonic (blue), as mentioned earlier. While the HOMO in the photoionization calculation shows a strong b-axis contribution for both the 19th and 25th harmonics, none of the HOMO or lower-lying orbitals show a particularly strong contribution from the a-axis. The photoionization calculation on its own is thus insufficient to explain the data.

However, looking at the combined photoionization and field ionization calculations, we see that the lower-lying orbitals do show a dominance of the a-axis for both harmonic energies. This points to field ionization as being crucial to fully explain the inversion of signal enhancement present in our data. We thus find that for some cases, a calculation of the photoionization cross section alone is insufficient to explain the data and that care should be taken when employing such a calculation on its own.

For clarity in the main text we limited our discussion to harmonics 19 and 25. However, we examined all harmonics to ensure that our analysis was consistent. In Supplementary Fig. 2 we show the combined photoionization and field ionization calculations as a function of energy over the whole energy range of the harmonics 19-33 shown in Fig. 2 of the main text. Supplementary Figure 2 shows that the dominance of the a-axis that we observe in the lower-lying orbitals 5b<sub>2</sub>, 4b<sub>2</sub> and 7a<sub>1</sub> is consistent throughout the energy range. Furthermore, it shows that the HOMO switches its dependence from the b-axis to the c-axis. Our analysis of the data shows a switch from the b-axis at lower harmonics to the a-axis at higher harmonics as shown in Fig. 3 of the main text. Thus, the explanation that the 19th harmonic receives a dominant signal from the 8a<sub>1</sub> orbital while the higher harmonics receive dominant signals from the 5b<sub>2</sub>, 4b<sub>2</sub> and 7a<sub>1</sub> is consistent with our analysis of all harmonics.

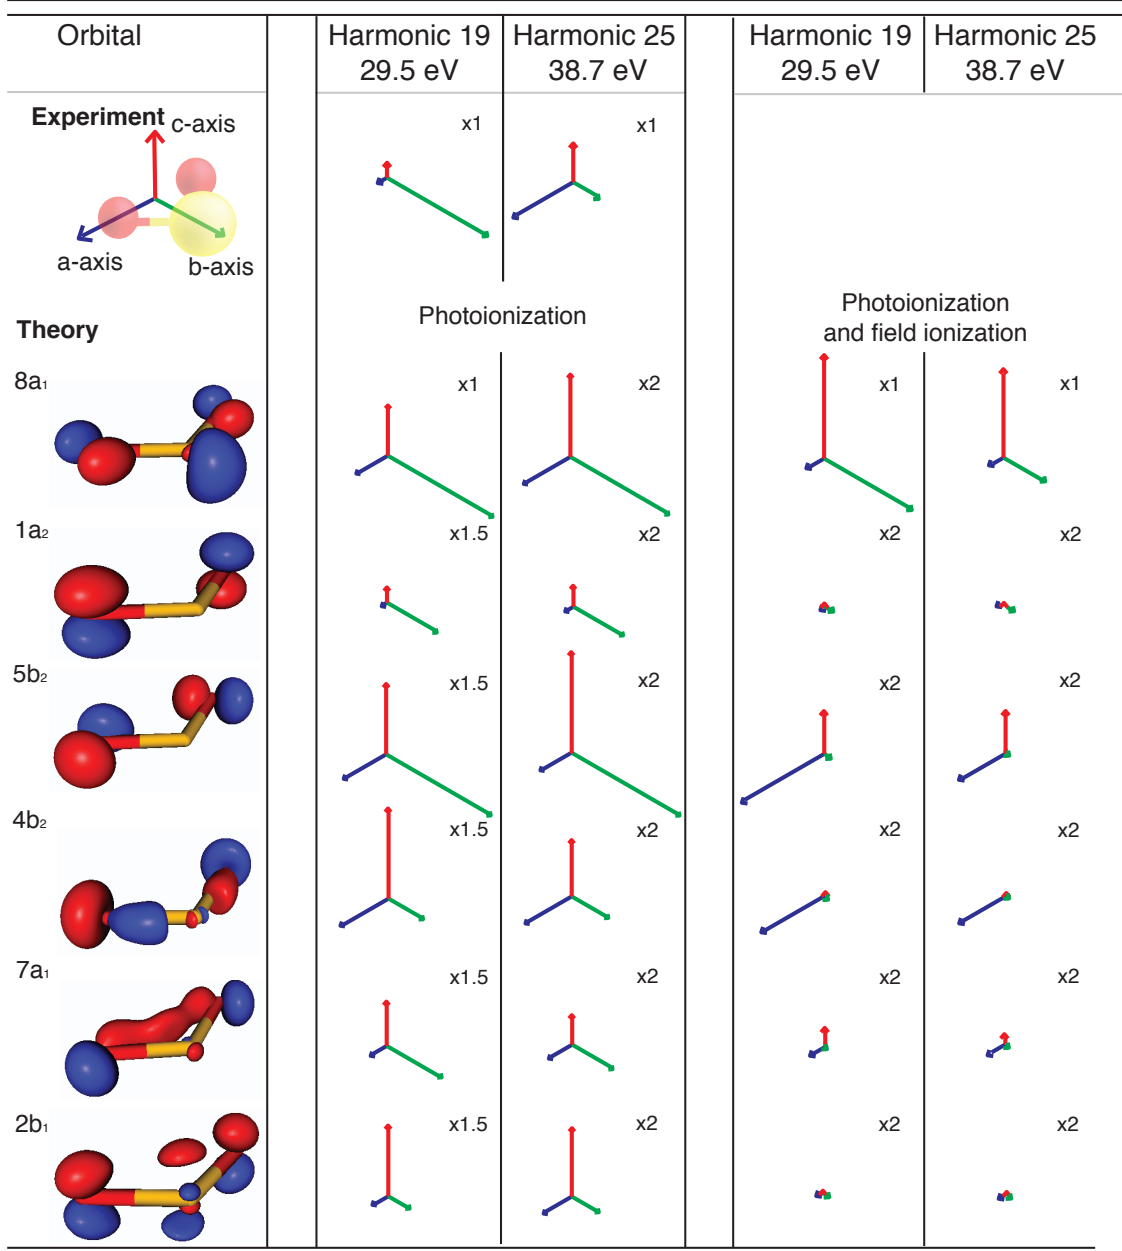

FIG. 1: Theoretical and experimental contributions to harmonic emission from all three molecular axes across the first few orbitals of SO<sub>2</sub> for harmonics 19 and 25. First row: the experiment shows a dominance of the b-axis for harmonic 19, but shows the b-axis as suppressed by the a-axis for harmonic 25. Middle columns: photoionization cross sections, which represent the recombination step of HHG. The b-axis provides a strong signal for many of the orbitals, but the a-axis never shows particular dominance. Right columns: photoionization cross sections are combined with field ionization calculations. The a-axis is strong and the b-axis suppressed for lower-lying orbitals 5b<sub>2</sub>, 4b<sub>2</sub> and 7a<sub>1</sub>. We thus find that we require the combined calculations of field ionization and photoionization to explain our data.

## II. CALCULATIONS OF PHOTOIONIZATION CROSS SECTIONS

To ensure that the recombination cross sections were accurately calculated and that the above was true, we calculated photoionization cross sections using two different methods, as mentioned in the main text. A comparison of the two methods is shown below in Supplementary Fig. 3. Supplementary Fig. 3a shows the first approach mentioned in the text based on the complex Kohn variational method, which was used in creating the combined probabilities

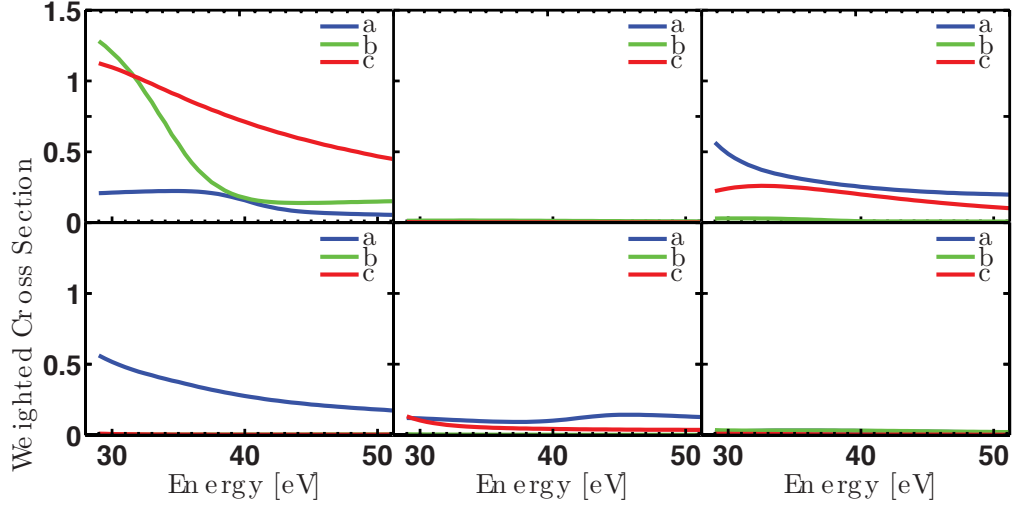

FIG. 2: A comparison of photoionization cross section calculations in two different methods. a) Method 1. b) Method 2. The minor differences do not influence the overall result when comparing to data or when combined with field ionization calculations.

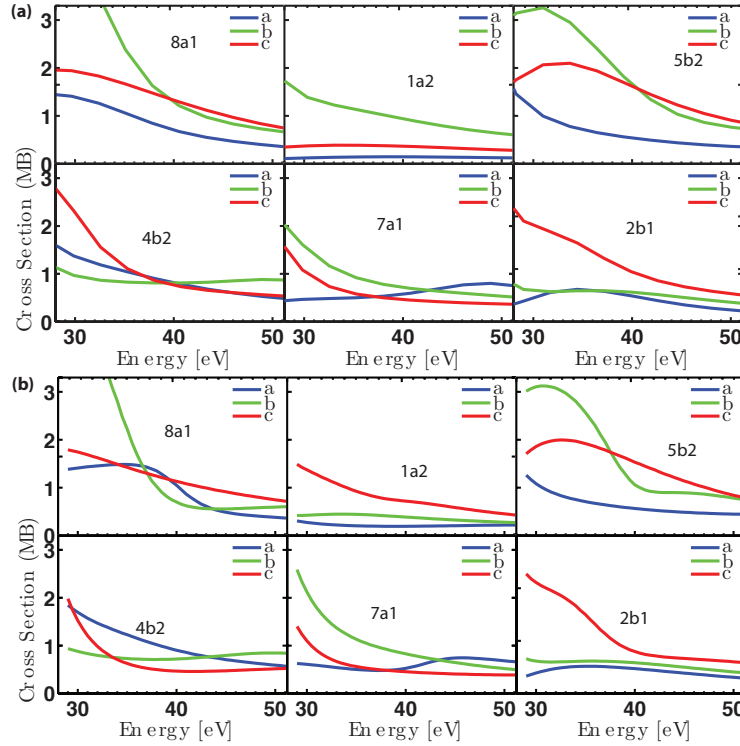

FIG. 3: A comparison of photoionization cross section calculations in two different methods. a) Method 1. b) Method 2. The minor differences do not influence the overall result when comparing to data or when combined with field ionization calculations.

in Fig. 4. Supplementary Fig. 3a shows the second approach mentioned in the text using the adopted DFT model. Although there are some differences between the calculations, they do not influence the overall result when comparing to the data or when combined with field ionization calculations.

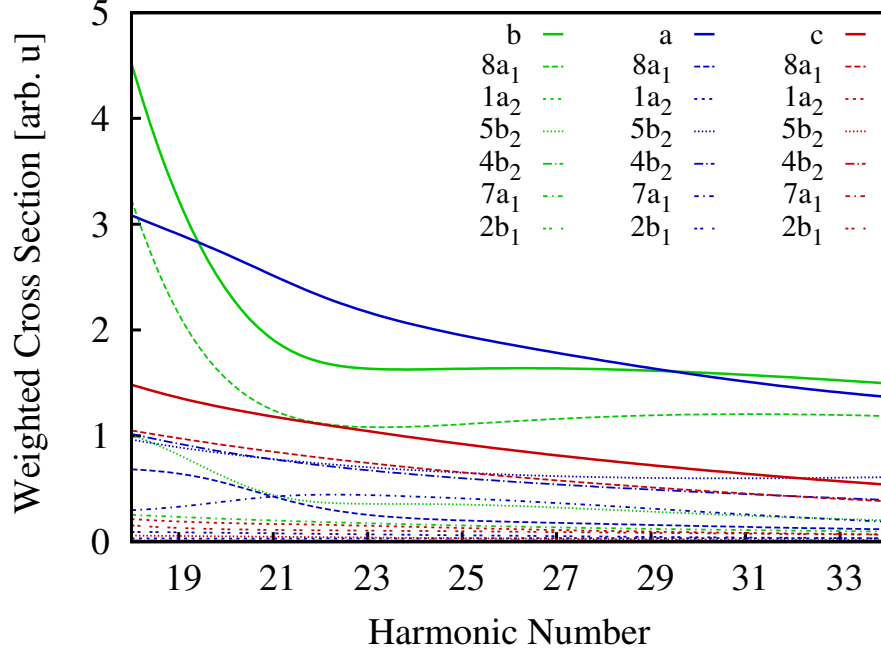

FIG. 4: SO<sub>2</sub> one photon ionization cross section sum weighted by the ionization yield at an intensity of  $2.6 \times 10^{14}$  W/cm<sup>2</sup>.

### III. EFFECTS OF LASER INTENSITY ON FIELD IONIZATION

Since the experimental laser intensity is a parameter that is not precisely known, we also consider the effects of laser intensity on the field ionization calculation based on the adopted DFT model. Figure 4 shows the result for the experimental peak intensity and using for the energy (HHG number) axis the ionization thresholds as they come out of the adopted DFT model. We see a turnover and from the change of relevance of the orbitals as discussed in the main text.

Figure ?? shows the same parameters as the Fig. 4, but now obtaining the energy axis using the experimental ionization thresholds. Fortunately, the main finding of the first graph does not change, although the crossing shifts slightly.

Figures 7, ??, 8 and 9 are similar to Fig. ??, but for different peak intensities of the laser. Evidently, the crossing of the blue and green curves moves with intensity, but it exists for quite some intensity range (although it disappears for lower intensities). Interestingly, one sees also that for higher intensities the red curve increases and shows a crossing with the green one, as in the experiment. However, we do not see a sharp decrease of the red curves for low HHG numbers, as seen in the experiment for high harmonic 19. Furthermore, one sees also that the blue and the green curves start to approach each other for higher HHG numbers, a similar trend as in the experiment.

We see the crossing due to lower lying orbitals confirmed, and the crossing position lies very close to the experimental one. Furthermore, the crossing and its position is intensity dependent, but it changes rather systematically with intensity and, again, it exists around the experimental intensity. In fact, the crossing of the green and the red curves seen in the experiment is somehow consistent with the calculation, although the intensities would be higher than the experimentally specified one.

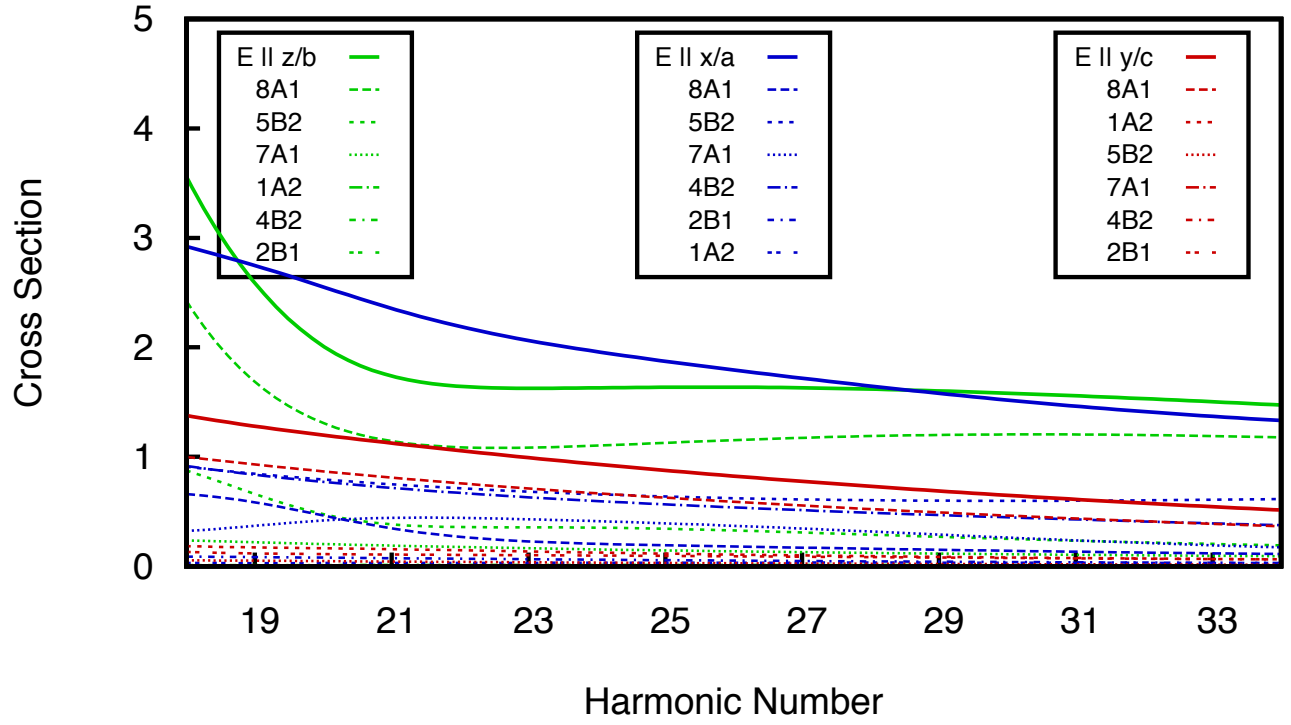

FIG. 5: SO<sub>2</sub> one photon ionization cross section sum weighted by the ionization yield at an intensity of  $2.6 \times 10^{14} \text{ W/cm}^2$  using experimental ionization potentials.

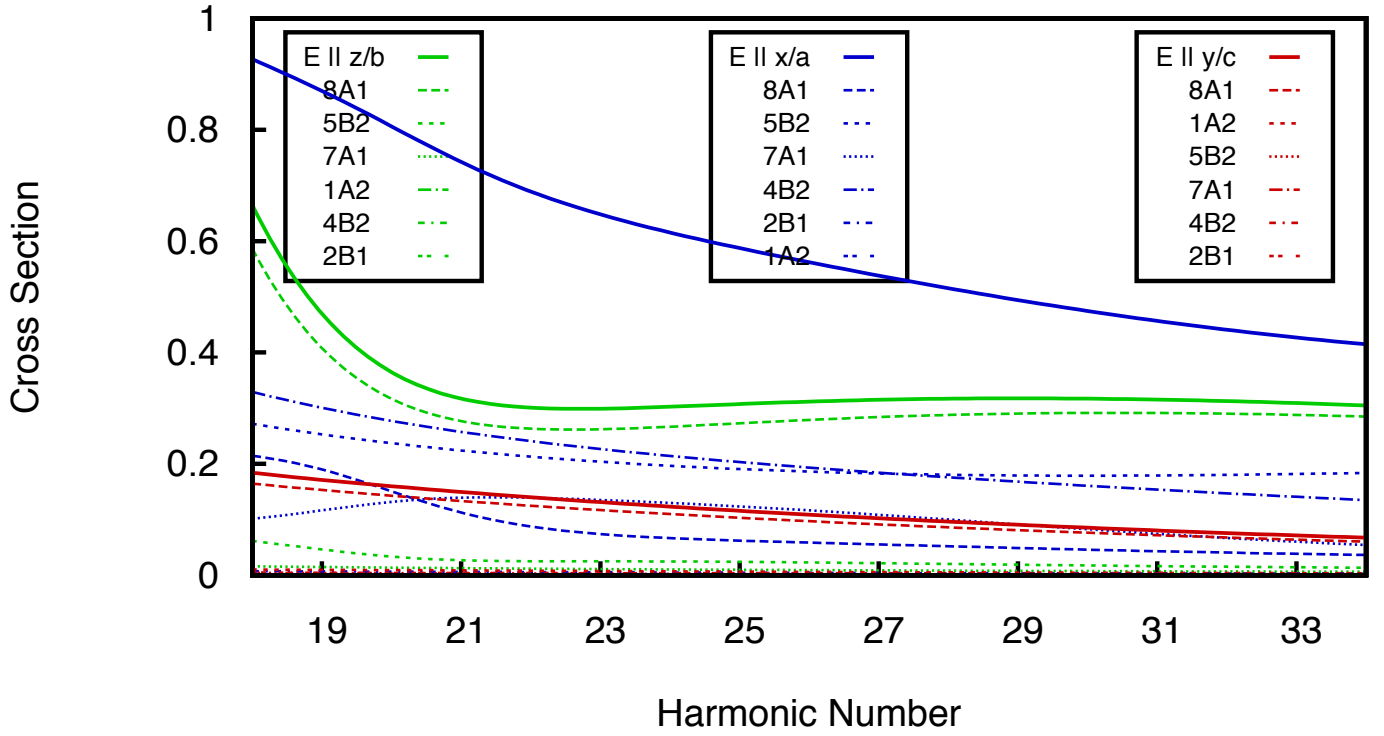

FIG. 6: SO<sub>2</sub> one photon ionization cross section sum weighted by the ionization yield at an intensity of  $1.5 \times 10^{14} \text{ W/cm}^2$  using experimental ionization potentials.

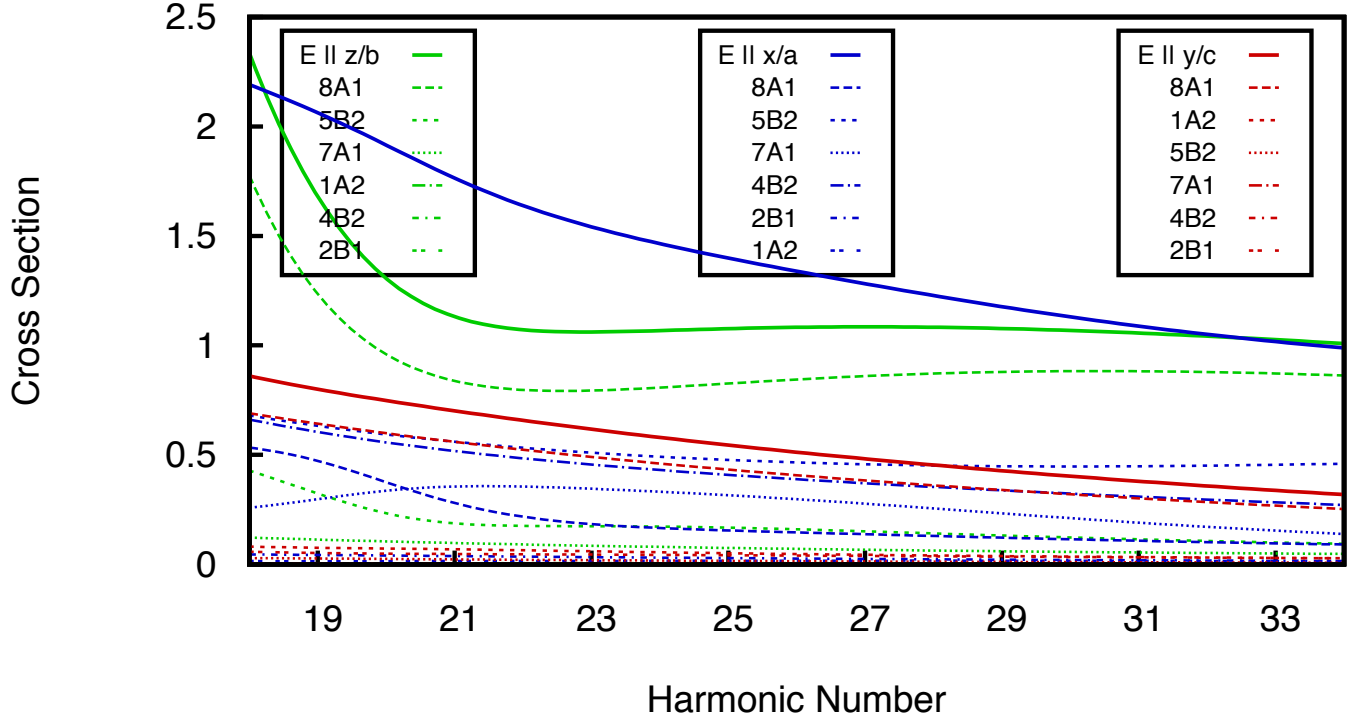

FIG. 7: SO<sub>2</sub> one photon ionization cross section sum weighted by the ionization yield at an intensity of  $2.2 \times 10^{14} \text{ W/cm}^2$  using experimental ionization potentials.

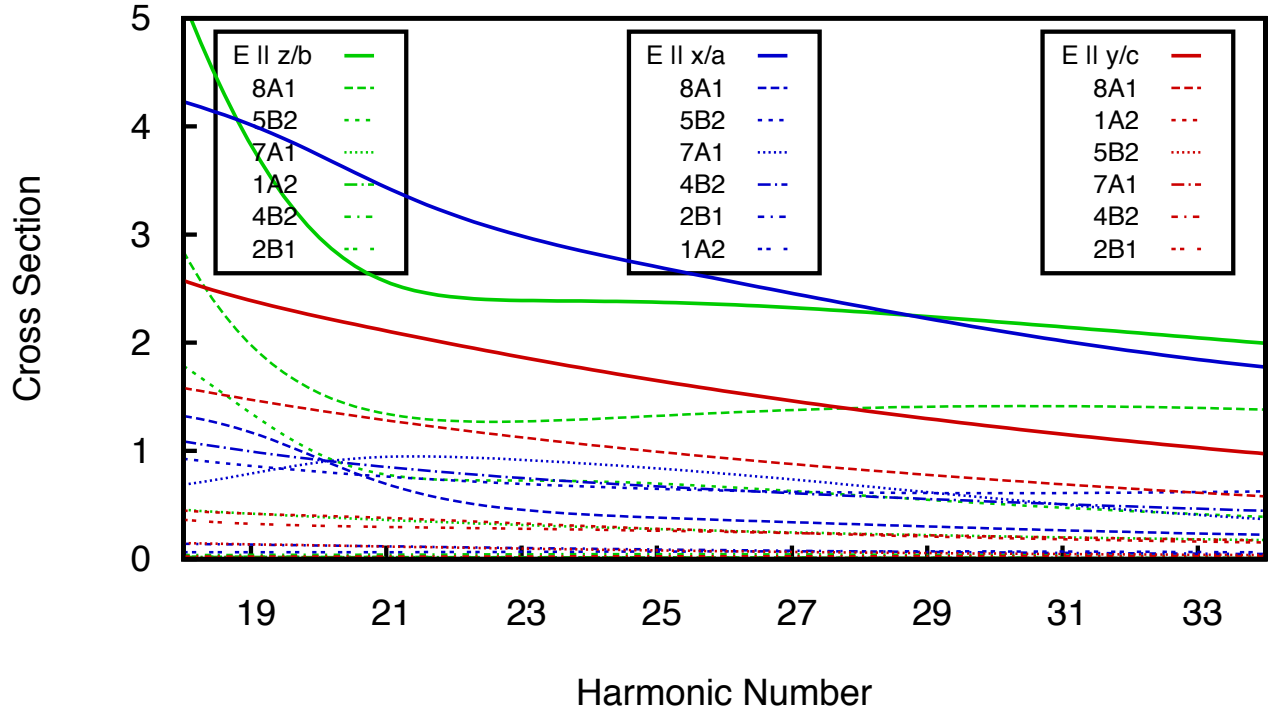

FIG. 8: SO<sub>2</sub> one photon ionization cross section sum weighted by the ionization yield at an intensity of  $3.2 \times 10^{14} \text{ W/cm}^2$  using experimental ionization potentials.

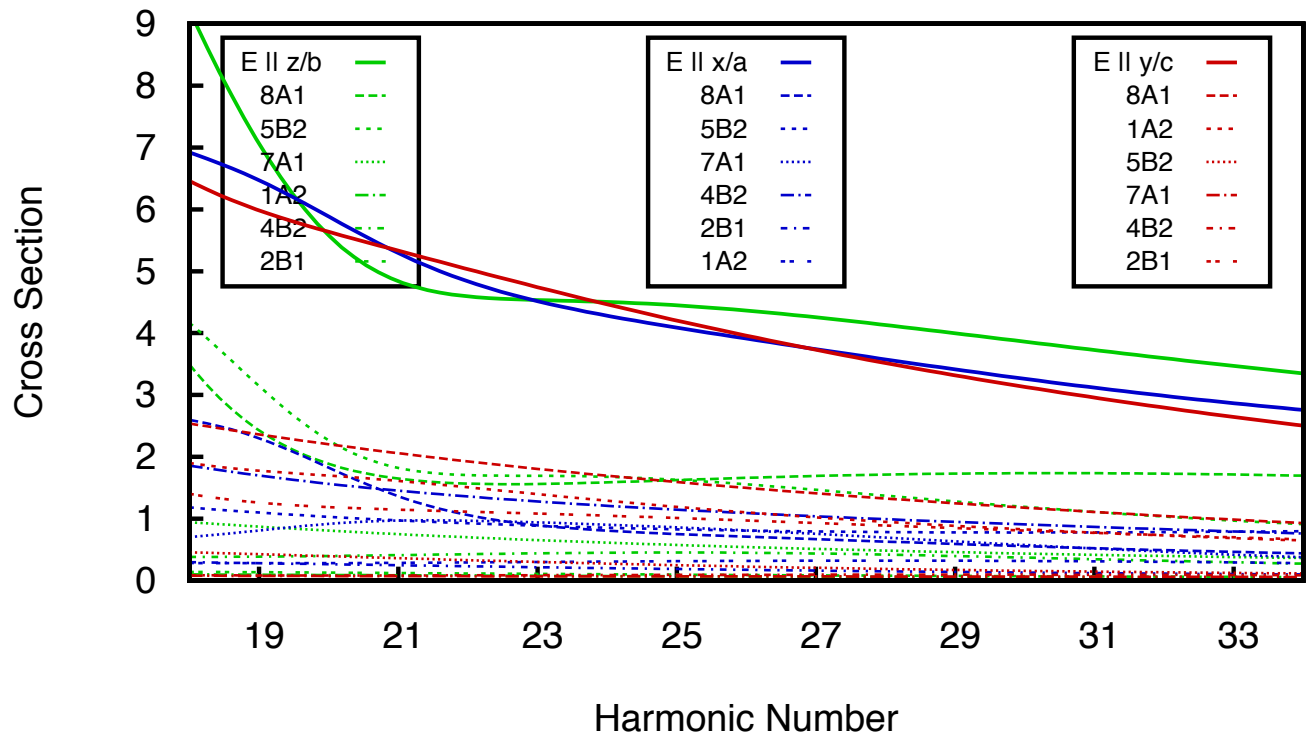

FIG. 9: SO<sub>2</sub> one photon ionization cross section sum weighted by the ionization yield at an intensity of  $4.7 \times 10^{14} \text{ W/cm}^2$  using experimental ionization potentials.
